# Supplementary material for: Developing machine-learned potentials to simultaneously capture the dynamics of excess protons and hydroxide ions in classical and path integral simulations
Source: arXiv:2308.06348 source file (2023-08-11)
Supplement: Supplementary file 1 [file SI.pdf]

# Supplementary Information for: Developing machine-learned potentials to simultaneously capture the dynamics of excess protons and hydroxide ions in classical and path integral simulations

Austin O. Atsango, Tobias Morawietz, and Thomas E. Markland*

*Department of Chemistry, Stanford University, Stanford, California, 94305, USA*

Ondrej Marsalek

*Faculty of Mathematics and Physics, Charles University, Prague, Czech Republic*

(Dated: August 11, 2023)

* tmarkland@stanford.edu

# I. RADIAL DISTRIBUTION FUNCTIONS

As an additional test of the accuracy of our GGA-trained MLP, we show here the H*-H (Fig. 1) and O*-H (Fig. 2) radial distribution functions (RDFs) for both the acid and base trajectories, with O* and H* defined in the main text as the O and H atoms that make up the $H_3O^+$ and $OH^-$ defects in simulations with an excess proton and a hydroxide ion respectively. Similar to the validation results presented in the main text, these RDFs focus on the proton defect environment and thus offer a stricter test of the performance of the MLP. In all cases, the GGA-trained MLP reproduces the *ab initio* RDF with almost quantitative accuracy.

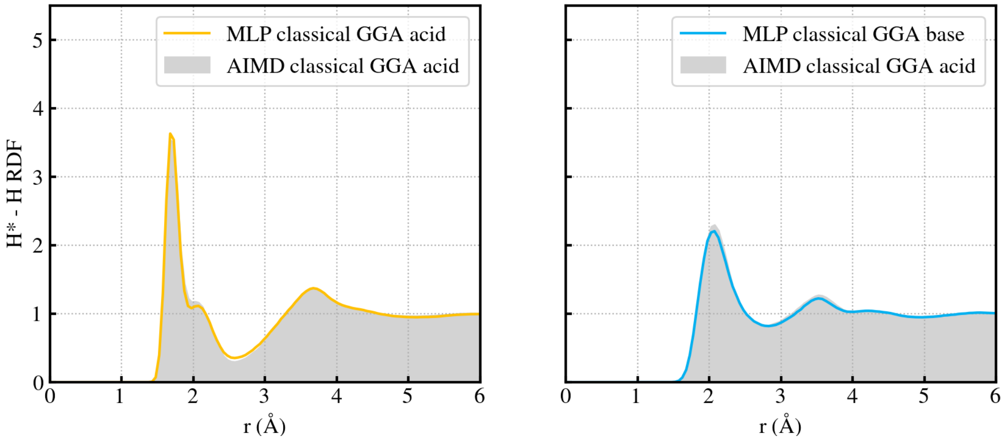


FIG. 1. Comparison of the H*H RDFs for revPBE-D3 AIMD and the revPBE-D3-trained MLP trajectories. The left panel shows this comparison for acid trajectories, while the right panel shows the comparison for base trajectories.

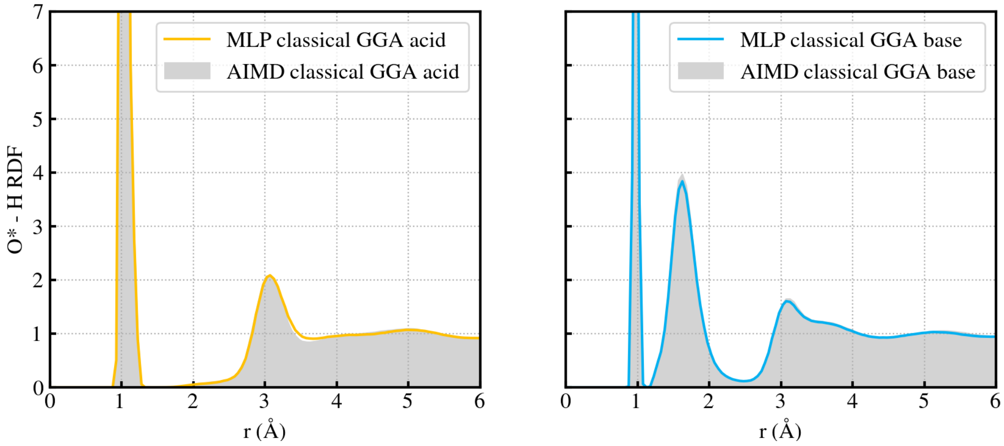


FIG. 2. Comparison of the O*H RDFs for revPBE-D3 AIMD and the revPBE-D3-trained MLP trajectories. The left panel shows this comparison for acid trajectories, while the right panel shows the comparison for base trajectories.

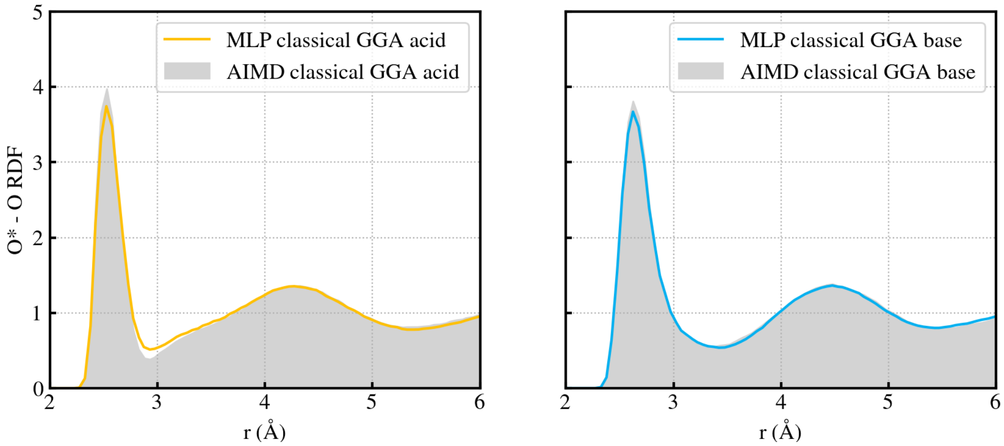


FIG. 3. Comparison of the O*O RDFs for revPBE-D3 AIMD and the revPBE-D3-trained MLP trajectories. The left panel shows this comparison for acid trajectories, while the right panel shows the comparison for base trajectories.

## II. VIBRATIONAL DENSITY OF STATES

The vibrational density of states (VDOS) for H* and O* shown in the main text are computed for their respective atoms only at frames when they are part of a proton defect. This is achieved by first obtaining a time-series of the velocity of the relevant atom and multiplying it by a 1.2 ps symmetric Hann window centered at the frame where the atom was part of a proton defect. This is done repeatedly for the defect atoms at different frames, and the resulting collection of 1.2 ps velocity segments is then used to compute velocity autocorrelation functions (VACFs). The VACFs are averaged and Fourier-transformed to yield a VDOS that encodes information about H* and O* but only in the brief time windows around when they were part of the proton defect [1].

For completeness, we present the unresolved H and O VDOS for the revPBE-D3 AIMD and revPBE-D3-trained MLP trajectories in Figures 4 and 5. These were obtained by simply generating velocity autocorrelation functions from the respective velocity time series and Fourier-transforming the result without the initial step of multiplying by a Hanning window. Similar to what is reported in the main text, the revPBE-D3-trained MLP trajectories reproduce the revPBE-D3 AIMD VDOS with almost quantitative accuracy.

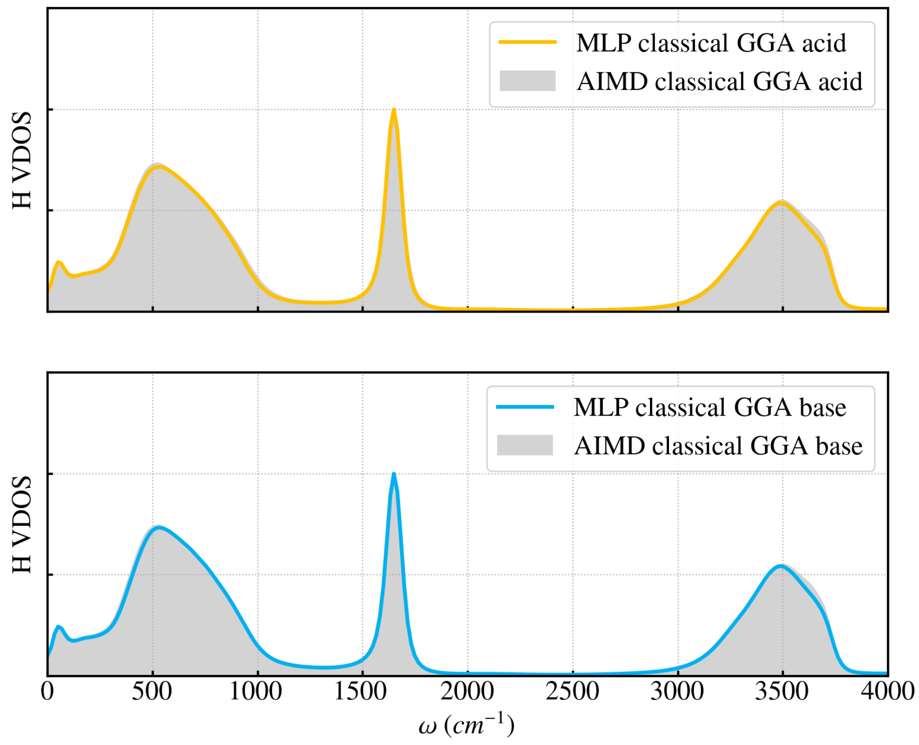


FIG. 4. Comparison of the H VDOS for revPBE-D3 AIMD and revPBE-D3-trained MLP trajectories. The top panel shows this comparison for acid trajectories, while the bottom panel shows the comparison for base trajectories.

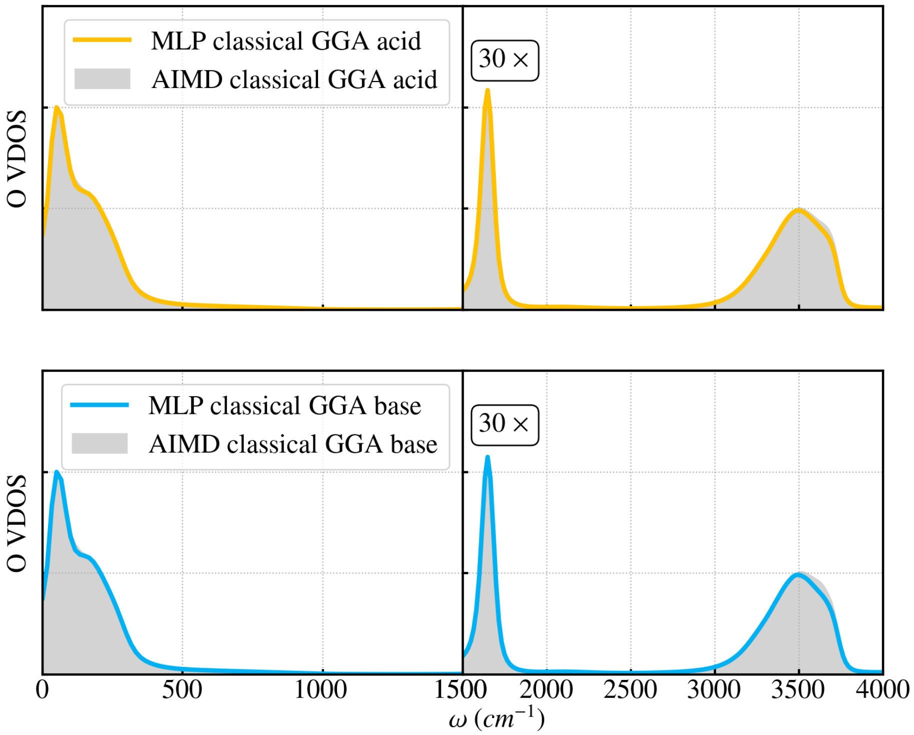


FIG. 5. Comparison of the O VDOS for revPBE-D3 AIMD and the revPBE-D3-trained MLP trajectories. The top panel shows this comparison for acid trajectories, while the bottom panel shows the comparison for base trajectories.

## III. DIFFUSION COEFFICIENTS

In addition to the full molecular and proton defect diffusion coefficients, Figure 6 in the main text also displays the vehicular component of the proton defect diffusion coefficient. This component is obtained by decomposing the full proton defect diffusion coefficient into its structural and vehicular parts, a process that is illustrated in Fig. 6 using a sample of X coordinates of $O^*$ ($X_{O^*}$). Our decomposition begins with the time series of the coordinates of $O^*$ (grey lines in Fig. 6). At each time step, the displacement of O* is either due to the molecular motion of the proton defect (vehicular diffusion) or to proton transfer reactions (structural diffusion), and these are placed in separate bins, resulting in a smooth trajectory of vehicular diffusion (red lines in Fig. 6) and a comparatively jagged trajectory of structural diffusion (blue lines in Fig. 6). The diffusion coefficients are then obtained from the mean squared displacement (MSD) of their respective trajectory.

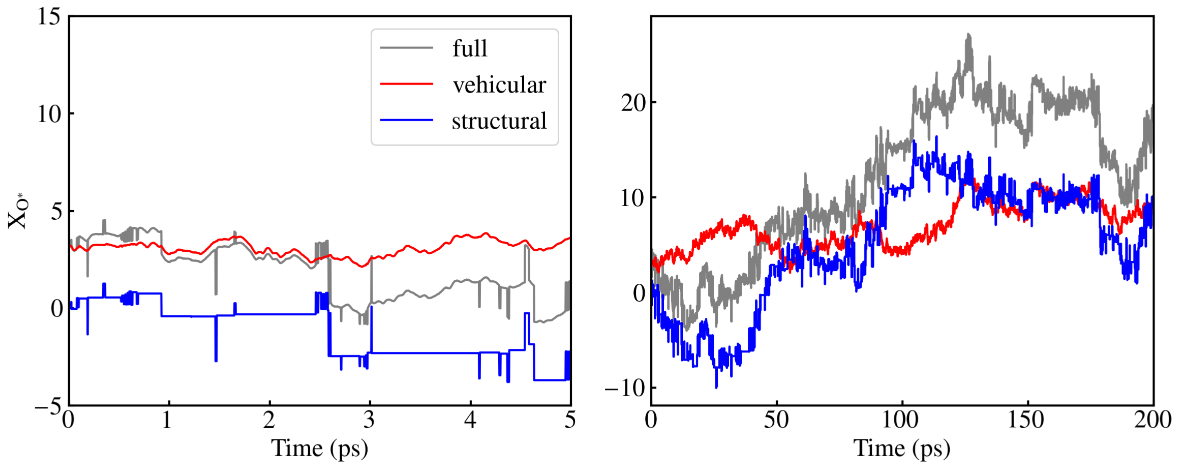


FIG. 6. An illustration of the decomposition of the proton defect trajectory into its structural and vehicular components

The molecular and proton defect (along with the structural and vehicular components) diffusion coefficients for MLP-based trajectories referenced in the main text are shown in Table I. The error bars are obtained from the standard deviation of the mean over independent 200 ps trajectories, and the diffusion coefficients are calculated by fitting the MSD curve in the 4 - 20 ps region. These values are based on periodic boxes containing 127 water molecules and 1 proton defect.

To investigate finite size effects, we also computed molecular and proton defect diffusion coefficients for systems containing a single proton defect and 127, 255, and 511 water molecules in cubic boxes of length 15.66 Å, 19.73 Å and 24.86 Å respectively using classical GGA MLP-based trajectories (Figure 8). These values are shown in Table II, with the error bars obtained as described above. From this data we observe that, as expected, the diffusion coefficients of water in both acid and base trajectories are inversely proportional to the box length [2], and they approach the experimental diffusion coefficient for pure water (2.41

| Nuclear representation | DFT Functional | Proton Defect | Diffusion Coefficients ($10^{-9}$ m$^2$/s) | | | |
|---|---|---|---|---|---|---|
| | | | Water (O) | O* Vehicular | O* Structural | O* |
| Classical | revPBE-D3 | $H_3O^+$ | 1.503 ± 0.001 | 1.309 ± 0.035 | 6.833 ± 0.203 | 8.043 ± 0.253 |
| | | $OH^-$ | 1.499 ± 0.001 | 1.093 ± 0.036 | 3.425 ± 0.136 | 4.947 ± 0.195 |
| | revPBE0-D3 | $H_3O^+$ | 2.222 ± 0.001 | 1.622 ± 0.046 | 6.358 ± 0.164 | 7.971 ± 0.208 |
| | | $OH^-$ | 2.189 ± 0.001 | 1.304 ± 0.038 | 1.890 ± 0.086 | 3.603 ± 0.133 |
| Quantum | revPBE-D3 | $H_3O^+$ | 1.039 ± 0.003 | 1.238 ± 0.087 | 12.051 ± 0.880 | 13.886 ± 1.081 |
| | | $OH^-$ | 1.016 ± 0.003 | 1.053 ± 0.115 | 10.572 ± 0.959 | 12.405 ± 1.110 |
| | revPBE0-D3 | $H_3O^+$ | 1.888 ± 0.002 | 1.751 ± 0.214 | 9.509 ± 0.786 | 10.916 ± 0.951 |
| | | $OH^-$ | 1.933 ± 0.003 | 1.712 ± 0.116 | 6.824 ± 0.551 | 9.244 ± 0.637 |

TABLE I. Water and charge defect diffusion coefficients for MLP acid and base trajectories containing 128 molecules, one of which is either $H_3O^+$ or $OH^-$

$\times\ 10^{-9}$ m$^2$/s) [3] as the system size is increased. Conversely, the proton defect diffusion coefficient exhibits little system-size dependence. The diffusion coefficients for the excess proton at different system sizes are all within each other's error bars, and the same trend is observed for all diffusion coefficients of the hydroxide ion except for the comparatively lower value at the 15.66 Å box length. Figure 8 also shows the structural components of the proton defect diffusion coefficient, and these closely follow the trend in the full proton defect diffusion coefficient, albeit with somewhat less system-size dependence. Overall, these trends are likely due to a combination of finite size and concentration-dependent effects: the proton defect concentrations are 0.43 M, 0.22 M, and 0.11 M for system sizes of 15.66 Å, 19.73 Å and 24.86 Å respectively. Due to these factors and the lack of a clear trend due to the size of the error bars (Figure 8), we do not include finite-size corrections in the proton defect diffusion coefficients reported in the manuscript (Figure 6).

| Charge Defect | Number of molecules | Diffusion Coefficients ($10^{-9}$ m$^2$/s) | | | |
|---|---|---|---|---|---|
| | | Water (O) | O* Vehicular | O* Structural | O* |
| $H_3O^+$ | 256 | 1.800 ± 0.001 | 1.385 ± 0.039 | 6.927 ± 0.217 | 8.344 ± 0.270 |
| | 512 | 1.935 ± 0.001 | 1.526 ± 0.065 | 6.876 ± 0.310 | 8.321 ± 0.401 |
| $OH^-$ | 256 | 1.801 ± 0.001 | 1.254 ± 0.036 | 3.981 ± 0.131 | 5.767 ± 0.178 |
| | 512 | 1.903 ± 0.001 | 1.321 ± 0.063 | 3.830 ± 0.170 | 5.834 ± 0.303 |

TABLE II. Water and charge defect diffusion coefficients for GGA MLP acid and base trajectories at varying system sizes

Figure 7 shows a detailed comparison of the diffusion coefficient values obtained from the classical GGA-trained MLP trajec-

tories with those obtained from GGA AIMD trajectories. All coefficients are obtained from 200-ps segments of the trajectory, and while AIMD values are displayed as single dotted lines, the more numerous (107 for acid and 70 for base) MLP values are displayed as a distribution. Both the acid and base plots show that all the AIMD diffusion coefficients are within the bounds of the distribution of the corresponding MLP diffusion coefficients. We can thus conclude that the GGA MLP reproduces the corresponding AIMD diffusion coefficient to within statistical accuracy.

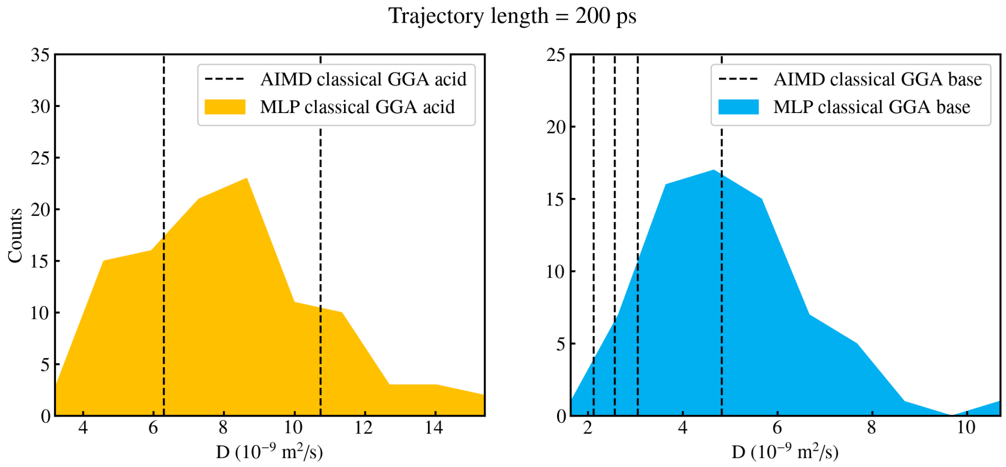


FIG. 7. A comparison of the distribution of proton defect diffusion coefficients obtained from MLP trajectories with the corresponding values obtained from AIMD trajectories. All sampled values are obtained from 200 ps-long trajectories.

Finally, Figures 9 and 10 show the mean squared displacement curves used to compute proton defect diffusion coefficients at different lengths of trajectory as discussed in Section V of the main manuscript.

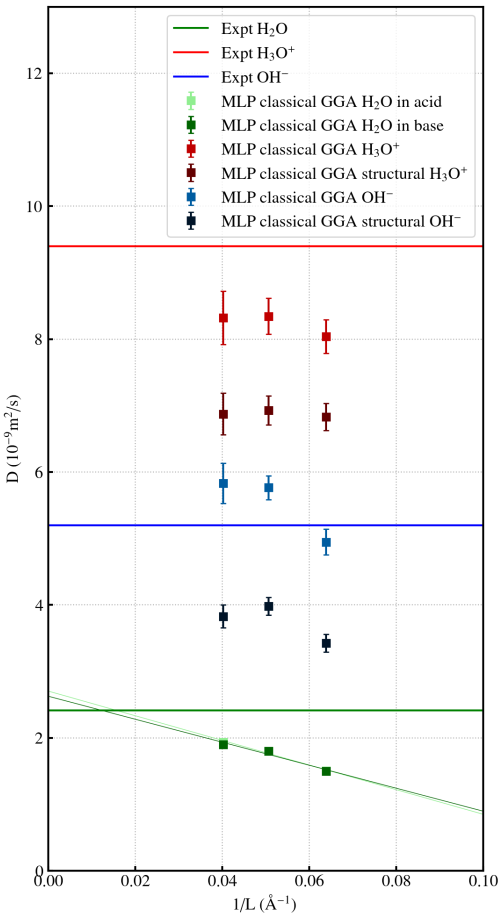


FIG. 8. Water and charge defect diffusion coefficients as functions of the inverse box length as calculated under a classical GGA MLP

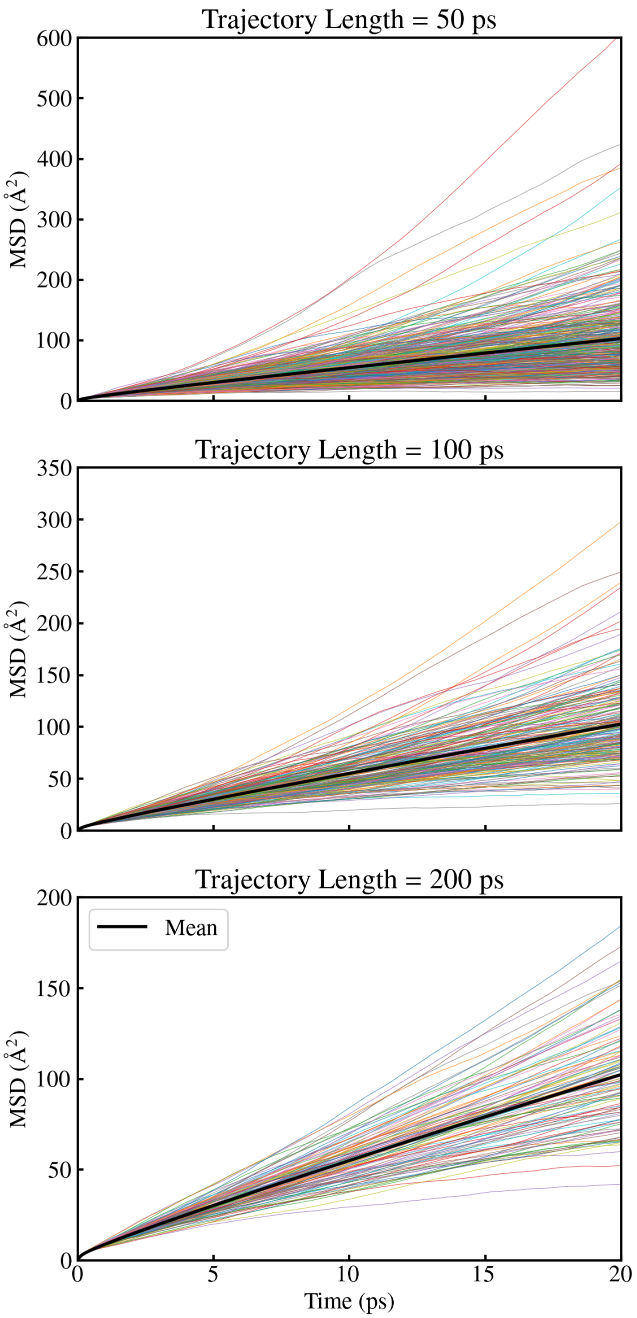


FIG. 9. Excess proton mean squared displacement curves obtained from the MLP GGA simulations computed at different trajectory lengths, with the corresponding means displayed as solid black lines. The reported diffusion coefficients are obtained as a linear fit to the 4-20 ps range.

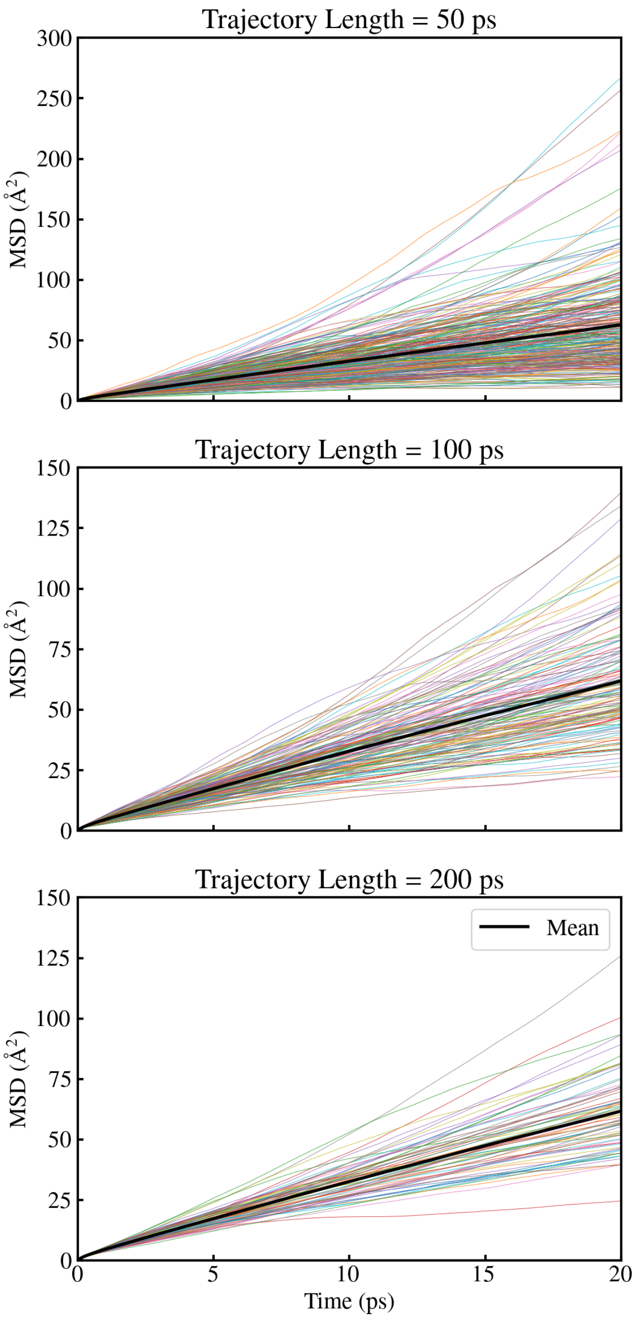


FIG. 10. Hydroxide ion mean squared displacement curves obtained from the MLP GGA simulations computed at different trajectory lengths, with the corresponding means displayed as solid black lines. The reported diffusion coefficients are obtained as a linear fit to the 4-20 ps range.

## IV. TRAINING SET AND LEARNING CURVES

As outlined in the main text, the details of the training set configuration are summarized in Table III. Additionally, the validation root mean square errors (RMSEs) for the revPBE-D3- and revPBE0-D3-trained MLPs are shown in Figs. 11 and 12.

| **Source** | **Simulation Temperature (K)** | **Criteria for selecting configurations** | **Nuclear representation in the source AIMD run** | **No. of configurations** |
|---|---|---|---|---|
| 50% random sample of dataset in Ref. 4 | 258 - 370 | Bulk water (N/A) | Classical + Quantum | 4594 |
| AIMD charge recombination runs | 300 | Uniform $\delta$ $H_3O^+$ | Classical | 3515 |
| | | | Quantum | 2280 |
| | | Uniform $\delta$ $OH^-$ | Classical | 9251 |
| | | | Quantum | 2707 |
| | 350 | Uniform $\delta$ $H_3O^+$ | Classical | 3496 |
| | | | Quantum | 3172 |
| | | Uniform $\delta$ $OH^-$ | Classical | 4200 |
| | | | Quantum | 3887 |
| **Total** | | | | **37102** |

TABLE III. A summary of the features of the training/validation set, including details of the AIMD runs where configurations were obtained, the criteria used to select the configurations, and the number of configurations obtained from each category.

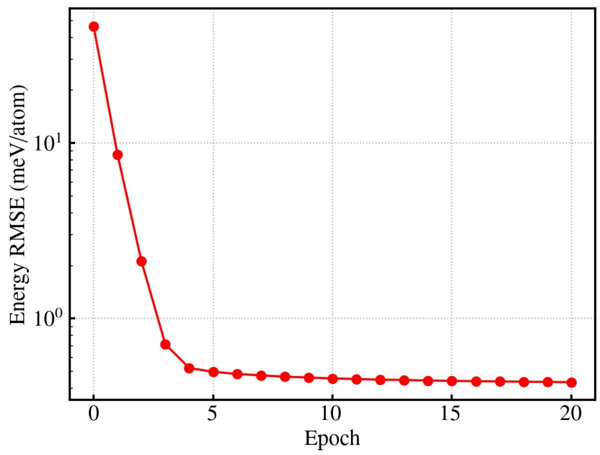


FIG. 11. Validation RMSE curve for the revPBE-D3-trained MLP

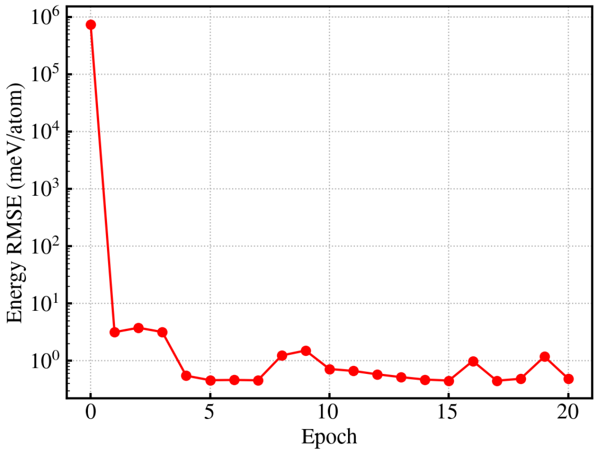


FIG. 12. Validation RMSE curve for the revPBE0-D3-trained MLP

[1] O. Marsalek and T. E. Markland, The Journal of Physical Chemistry Letters **8**, 1545 (2017).

[2] I.-C. Yeh and G. Hummer, The Journal of Physical Chemistry B **108**, 15873 (2004).

[3] M. Holz, S. R. Heil, and A. Sacco, Physical Chemistry Chemical Physics **2**, 4740 (2000).

[4] T. Morawietz, O. Marsalek, S. R. Pattenaude, L. M. Streacker, D. Ben-Amotz, and T. E. Markland, The Journal of Physical Chemistry Letters **9**, 851 (2018).
